# Supplementary material for: Fairness Improves Learning from Noisily Labeled Long-Tailed Data
Source: arXiv:2303.12291 source file (2023-03-22)
Supplement: Supplementary file 1 [file proofs.tex]

\section{Omitted proofs}
